# Supplementary material for: HomoMatcher: Dense Feature Matching Results with Semi-Dense Efficiency by Homography Estimation
Source: arXiv:2411.06700 source file (2024-11-11)
Supplement: Supplementary file 1 [file 7-Appendix.tex]

\section*{\LARGE Supplementary Materials}  % The '*' makes the section unnumbered

\section{Theoretical Foundations for Optimizing Homography}
